# Supplementary material for: Federated Learning for Data Streams
Source: arXiv:2301.01542 source file (2023-01-04)
Supplement: Supplementary file 1 [file simulator.tex]

We simulate the arrival process at every client as a (potentially non-homogeneous) Poisson process with intensity function / arrival rate $\lambda_{t}, t>0$. We consider different forms of arrival processes to simulate different plausible data streams:
\begin{enumerate}
    \item Constant: $\lambda_{t} \equiv \lambda_{0}$
    \item Single impulse:  $\lambda_{t} = a_{0} \cdot \mathds{1}\left\{t=0\right\}$ where $a_{0} \in \mathbb{R}^{+}$ is the intensity of the arrival process.
    \item Periodic arrival rate: $\lambda_{t} = a_{0} \cdot \mathds{1}\left\{t=0~\text{mod}~\tau \right\}$, where $\tau>0$ is the period of the arrival process and $a_{0} \in \mathbb{R}^{+}$ is the intensity of the arrival process. It corresponds to the average number of points received in one period.
\end{enumerate}
