# Supplementary material for: Federated Learning for Data Streams
Source: arXiv:2301.01542 source file (2023-01-04)
Supplement: Supplementary file 2 [file toy.tex]

\begin{figure}
    \centering
    \includegraphics[scale=0.3]{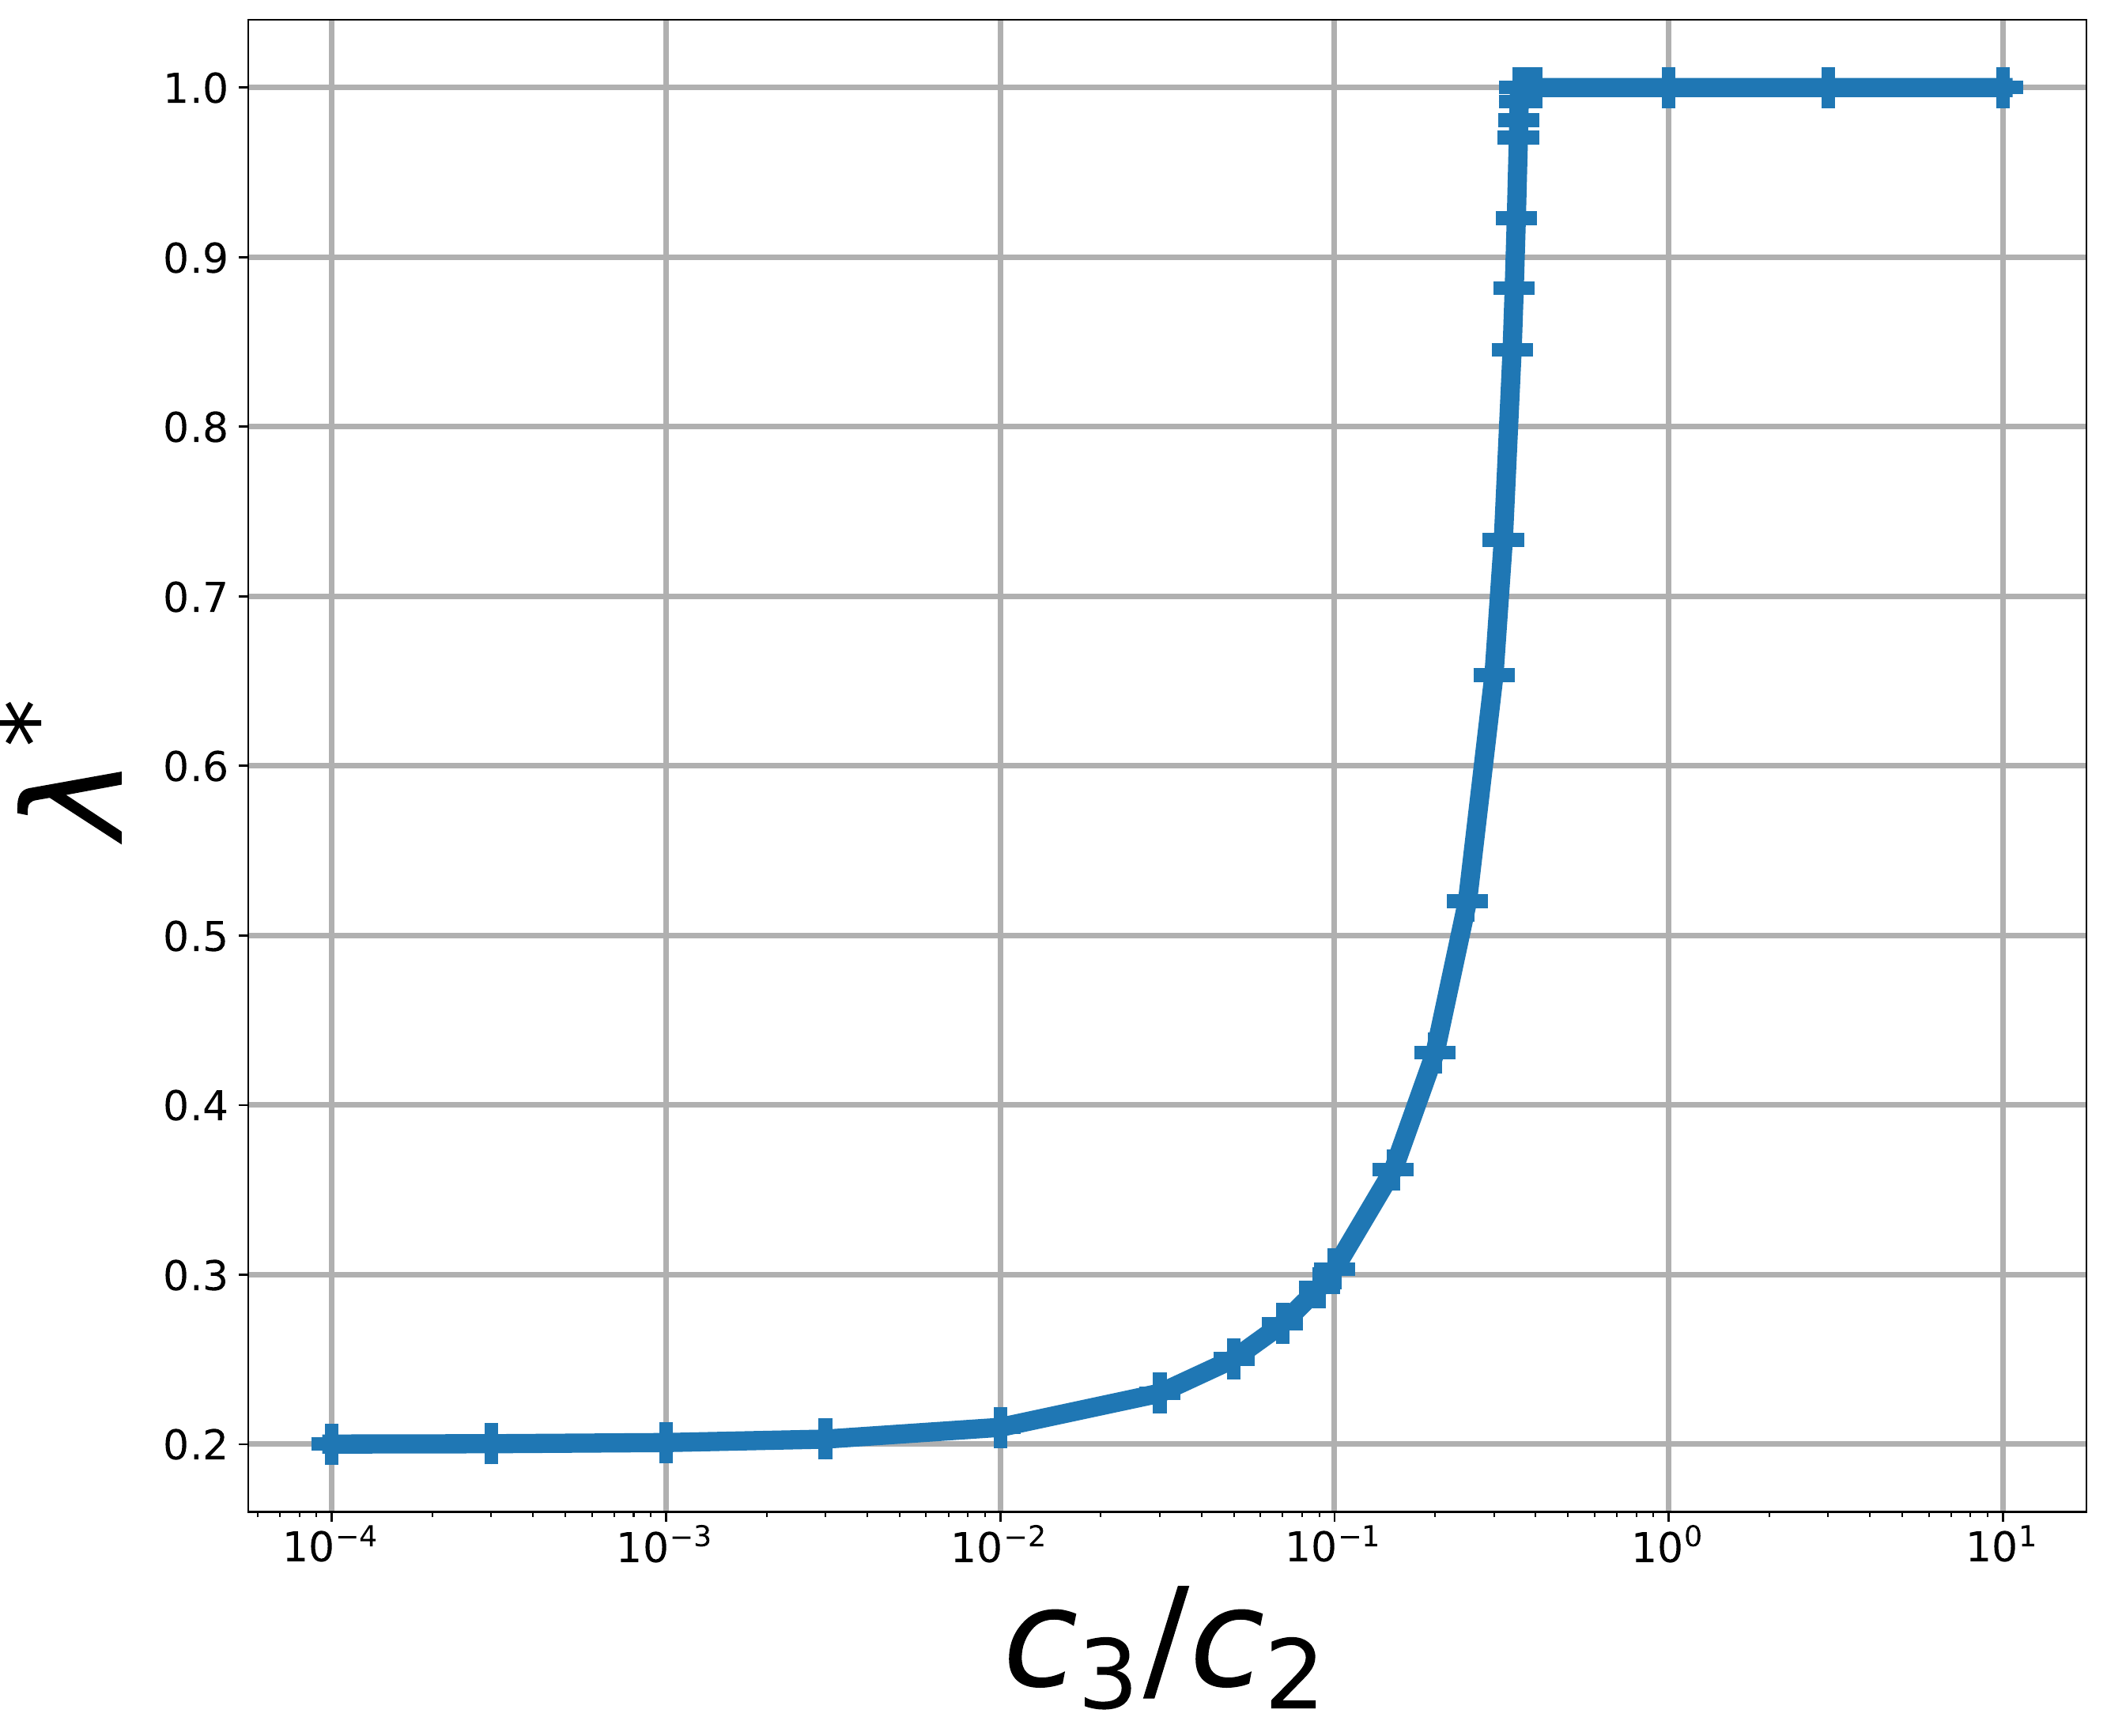}
    \caption{Effect of the ratio $c_{3}/ c_{2}$ on $\bm{\lambda}^{*}$}
    \label{fig:objective_weights_effect}
\end{figure}
